# Supplementary material for: Uncertainty separation via ensemble quantile regression
Source: arXiv:2412.13738 source file (2024-12-18)
Supplement: Supplementary file 1 [file Appendix.tex]

\section{Appendix}
\subsection{Relation Between Quantile Difference and Variance}
\label{sec:q_vs_sigma}

(\Navid{to be double checked}) We aim to find the value of $\alpha$ such that the following relationship holds:

\begin{equation} \sigma_{\text{total}}(x) = \frac{1}{N} \sum_{i=1}^{N} \left( q_{1-\alpha}^{(i)}(x) - q_{\alpha}^{(i)}(x) \right), \label{eq
} \end{equation}

where $\sigma_{\text{total}}(x)$ is the standard deviation of the variable $x$, and $q_{\alpha}^{(i)}(x)$ denotes the $\alpha$-quantile of the $i$-th sample.

Assuming that $x$ follows a normal distribution $\mathcal{N}(\mu, \sigma^2)$, the $\alpha$-quantile is given by:

\begin{equation} q_{\alpha} = \mu + z_{\alpha} \sigma, \label{eq
} \end{equation}

where $z_{\alpha}$ is the $\alpha$-quantile of the standard normal distribution $Z \sim \mathcal{N}(0, 1)$.

Due to the symmetry of the standard normal distribution:

\begin{equation} z_{1 - \alpha} = -z_{\alpha}. \label{eq
} \end{equation}

Using Equations \eqref{eq
} and \eqref{eq
}, the difference between the $(1 - \alpha)$-quantile and the $\alpha$-quantile is:

\begin{align} q_{1 - \alpha} - q_{\alpha} &= \left( \mu + z_{1 - \alpha} \sigma \right) - \left( \mu + z_{\alpha} \sigma \right) \notag \ &= \left( \mu - z_{\alpha} \sigma \right) - \left( \mu + z_{\alpha} \sigma \right) \notag \ &= -2 z_{\alpha} \sigma. \label{eq
} \end{align}

Since $z_{\alpha} < 0$ for $\alpha < 0.5$, we have:

\begin{equation} q_{1 - \alpha} - q_{\alpha} = 2 | z_{\alpha} | \sigma. \label{eq
} \end{equation}

Substituting Equation \eqref{eq
} into Equation \eqref{eq
}, we require:

\begin{equation} \sigma = 2 | z_{\alpha} | \sigma. \label{eq
} \end{equation}

Dividing both sides of Equation \eqref{eq
} by $\sigma$ (assuming $\sigma \neq 0$):

\begin{equation} 1 = 2 | z_{\alpha} |. \label{eq
} \end{equation}

Solving for $| z_{\alpha} |$:

\begin{equation} | z_{\alpha} | = \frac{1}{2}. \label{eq
} \end{equation}

Using the cumulative distribution function (CDF) of the standard normal distribution, the value of $\alpha$ corresponding to $z_{\alpha} = -\frac{1}{2}$ is:

\begin{align} \alpha &= \Phi\left( -\frac{1}{2} \right) \notag \ &= 1 - \Phi\left( \frac{1}{2} \right) \notag \ &\approx 1 - 0.6915 \notag \ &= 0.3085. \label{eq
} \end{align}

\textbf{Conclusion:} When $\alpha \approx 0.3085$, the average difference between the $(1 - \alpha)$-quantile and the $\alpha$-quantile equals the standard deviation $\sigma$:

\begin{equation} \sigma_{\text{total}}(x) = \frac{1}{N} \sum_{i=1}^{N} \left( q_{1 - 0.3085}^{(i)}(x) - q_{0.3085}^{(i)}(x) \right). \end{equation}

This establishes the relationship between the quantile difference and the variance for a normally distributed variable $x$.
